# Supplementary material for: Are the different layers of a social network conveying the same information?
Source: arXiv:1801.02874 ancillary file (2018-01-09)
Supplement: Supplementary file 1 [file SI_article.pdf]

# Are the different layers of a social network conveying the same information?

Ajaykumar Manivannan, W. Quin Yow, Roland Bouffanais, Alain Barrat

Full list of author information is available at the end of the article

## 1 Comparison between term-aggregated networks

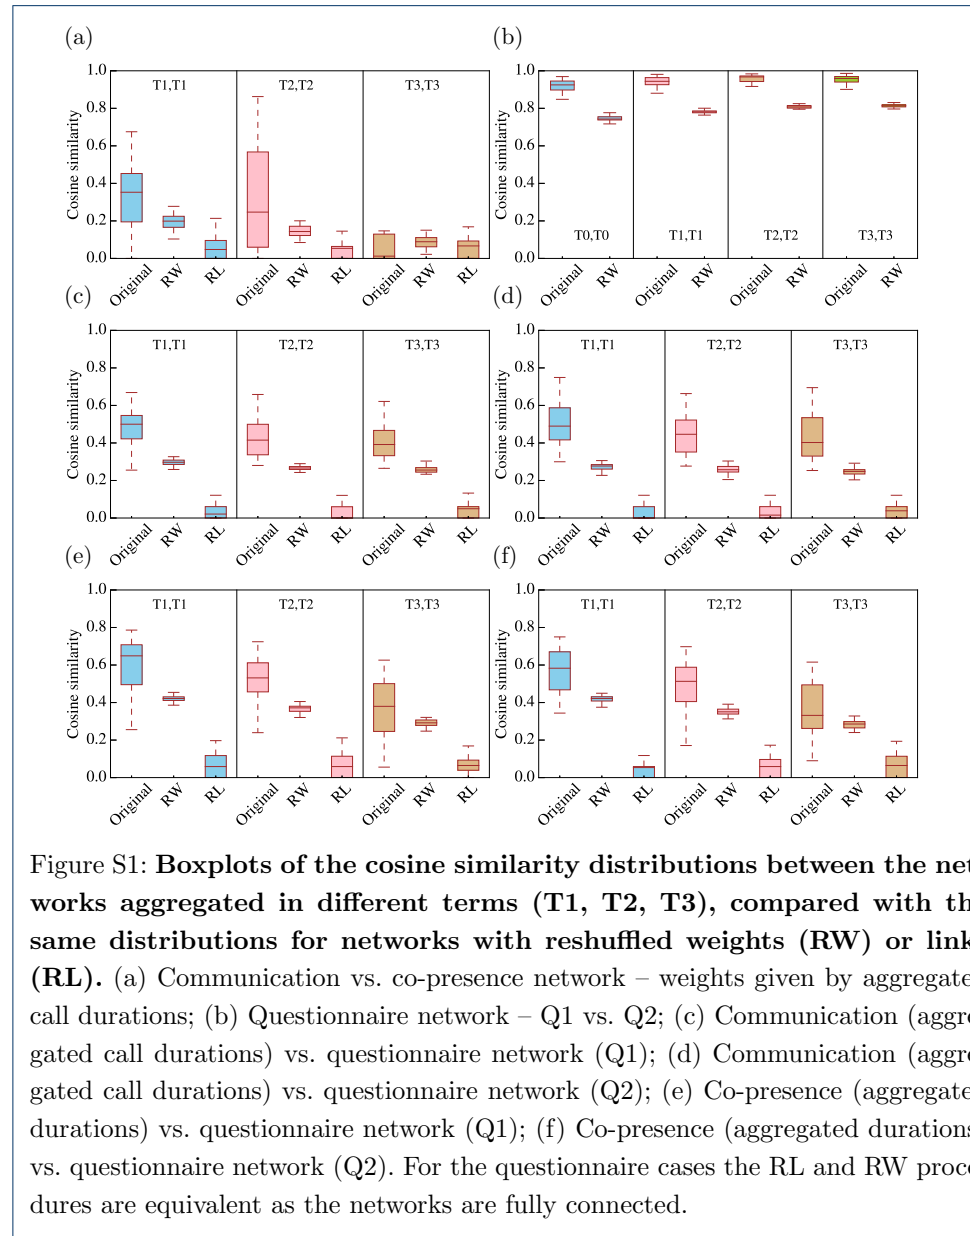

Table S1: Pearson correlation coefficients between term-aggregated networks

(a) Communication vs. co-presence.

|             | Duration-T1        | Duration-T2        | Duration-T3        | Number-T1          | Number-T2          | Number-T3          |
|-------------|--------------------|--------------------|--------------------|--------------------|--------------------|--------------------|
| Duration-T1 | -0.02<br>(p=0.863) | -0.14<br>(p=0.262) | 0.06<br>(p=0.76)   | -0.02<br>(p=0.865) | -0.09<br>(p=0.483) | 0.21<br>(p=0.285)  |
| Duration-T2 | 0.06<br>(p=0.58)   | 0.16<br>(p=0.181)  | 0.07<br>(p=0.737)  | 0.02<br>(p=0.866)  | 0.17<br>(p=0.165)  | 0.12<br>(p=0.558)  |
| Duration-T3 | 0.04<br>(p=0.722)  | 0.14<br>(p=0.29)   | -0.07<br>(p=0.735) | 0.01<br>(p=0.936)  | 0.13<br>(p=0.324)  | -0.07<br>(p=0.744) |
| Number-T1   | 0.02<br>(p=0.879)  | -0.17<br>(p=0.174) | 0.03<br>(p=0.864)  | 0.01<br>(p=0.903)  | -0.16<br>(p=0.216) | 0.27<br>(p=0.159)  |
| Number-T2   | 0.1<br>(p=0.384)   | 0.27<br>(p=0.027)  | 0.05<br>(p=0.793)  | 0.06<br>(p=0.621)  | 0.27<br>(p=0.027)  | 0.08<br>(p=0.672)  |
| Number-T3   | 0.12<br>(p=0.293)  | 0.24<br>(p=0.066)  | -0.07<br>(p=0.734) | 0.08<br>(p=0.5)    | 0.21<br>(p=0.109)  | -0.08<br>(p=0.694) |

(b) Communication vs. Questionnaire

|             | Q1-T0             | Q1-T1             | Q1-T2             | Q1-T3             | Q2-T0             | Q2-T1             | Q2-T2             | Q2-T3             |
|-------------|-------------------|-------------------|-------------------|-------------------|-------------------|-------------------|-------------------|-------------------|
| Duration-T1 | 0.28<br>(p=0.0)   | 0.31<br>(p=0.0)   | 0.24<br>(p=0.002) | 0.23<br>(p=0.003) | 0.38<br>(p=0.0)   | 0.25<br>(p=0.002) | 0.31<br>(p=0.0)   | 0.21<br>(p=0.007) |
| Duration-T2 | 0.27<br>(p=0.001) | 0.29<br>(p=0.0)   | 0.3<br>(p=0.0)    | 0.35<br>(p=0.0)   | 0.27<br>(p=0.001) | 0.34<br>(p=0.0)   | 0.37<br>(p=0.0)   | 0.3<br>(p=0.0)    |
| Duration-T3 | 0.22<br>(p=0.013) | 0.28<br>(p=0.001) | 0.25<br>(p=0.005) | 0.22<br>(p=0.013) | 0.31<br>(p=0.0)   | 0.3<br>(p=0.001)  | 0.33<br>(p=0.0)   | 0.24<br>(p=0.007) |
| Number-T1   | 0.25<br>(p=0.001) | 0.25<br>(p=0.001) | 0.22<br>(p=0.005) | 0.15<br>(p=0.054) | 0.3<br>(p=0.0)    | 0.17<br>(p=0.031) | 0.27<br>(p=0.001) | 0.13<br>(p=0.09)  |
| Number-T2   | 0.24<br>(p=0.003) | 0.24<br>(p=0.004) | 0.26<br>(p=0.001) | 0.31<br>(p=0.0)   | 0.24<br>(p=0.003) | 0.25<br>(p=0.002) | 0.32<br>(p=0.0)   | 0.26<br>(p=0.001) |
| Number-T3   | 0.23<br>(p=0.009) | 0.26<br>(p=0.003) | 0.26<br>(p=0.003) | 0.19<br>(p=0.029) | 0.34<br>(p=0.0)   | 0.25<br>(p=0.004) | 0.34<br>(p=0.0)   | 0.22<br>(p=0.011) |

(c) Co-presence vs. questionnaire.

|             | Q1-T0             | Q1-T1             | Q1-T2             | Q1-T3              | Q2-T0             | Q2-T1             | Q2-T2             | Q2-T3             |
|-------------|-------------------|-------------------|-------------------|--------------------|-------------------|-------------------|-------------------|-------------------|
| Duration-T1 | 0.27<br>(p=0.0)   | 0.32<br>(p=0.0)   | 0.35<br>(p=0.0)   | 0.3<br>(p=0.0)     | 0.14<br>(p=0.008) | 0.2<br>(p=0.0)    | 0.26<br>(p=0.0)   | 0.22<br>(p=0.0)   |
| Duration-T2 | 0.15<br>(p=0.011) | 0.31<br>(p=0.0)   | 0.26<br>(p=0.0)   | 0.3<br>(p=0.0)     | 0.09<br>(p=0.106) | 0.2<br>(p=0.001)  | 0.17<br>(p=0.004) | 0.26<br>(p=0.0)   |
| Duration-T3 | 0.12<br>(p=0.152) | 0.2<br>(p=0.016)  | 0.18<br>(p=0.027) | 0.18<br>(p=0.032)  | 0.18<br>(p=0.03)  | 0.1<br>(p=0.24)   | 0.18<br>(p=0.028) | 0.2<br>(p=0.017)  |
| Number-T1   | 0.2<br>(p=0.0)    | 0.21<br>(p=0.0)   | 0.24<br>(p=0.0)   | 0.19<br>(p=0.001)  | 0.15<br>(p=0.005) | 0.13<br>(p=0.014) | 0.19<br>(p=0.001) | 0.12<br>(p=0.034) |
| Number-T2   | 0.13<br>(p=0.028) | 0.21<br>(p=0.0)   | 0.16<br>(p=0.007) | 0.2<br>(p=0.001)   | 0.07<br>(p=0.202) | 0.14<br>(p=0.017) | 0.08<br>(p=0.171) | 0.18<br>(p=0.002) |
| Number-T3   | 0.04<br>(p=0.669) | 0.06<br>(p=0.496) | 0.01<br>(p=0.886) | -0.02<br>(p=0.788) | 0.14<br>(p=0.105) | 0.02<br>(p=0.767) | 0.05<br>(p=0.586) | 0.06<br>(p=0.454) |

## 2 Homophily patterns in the yearly aggregated co-presence network

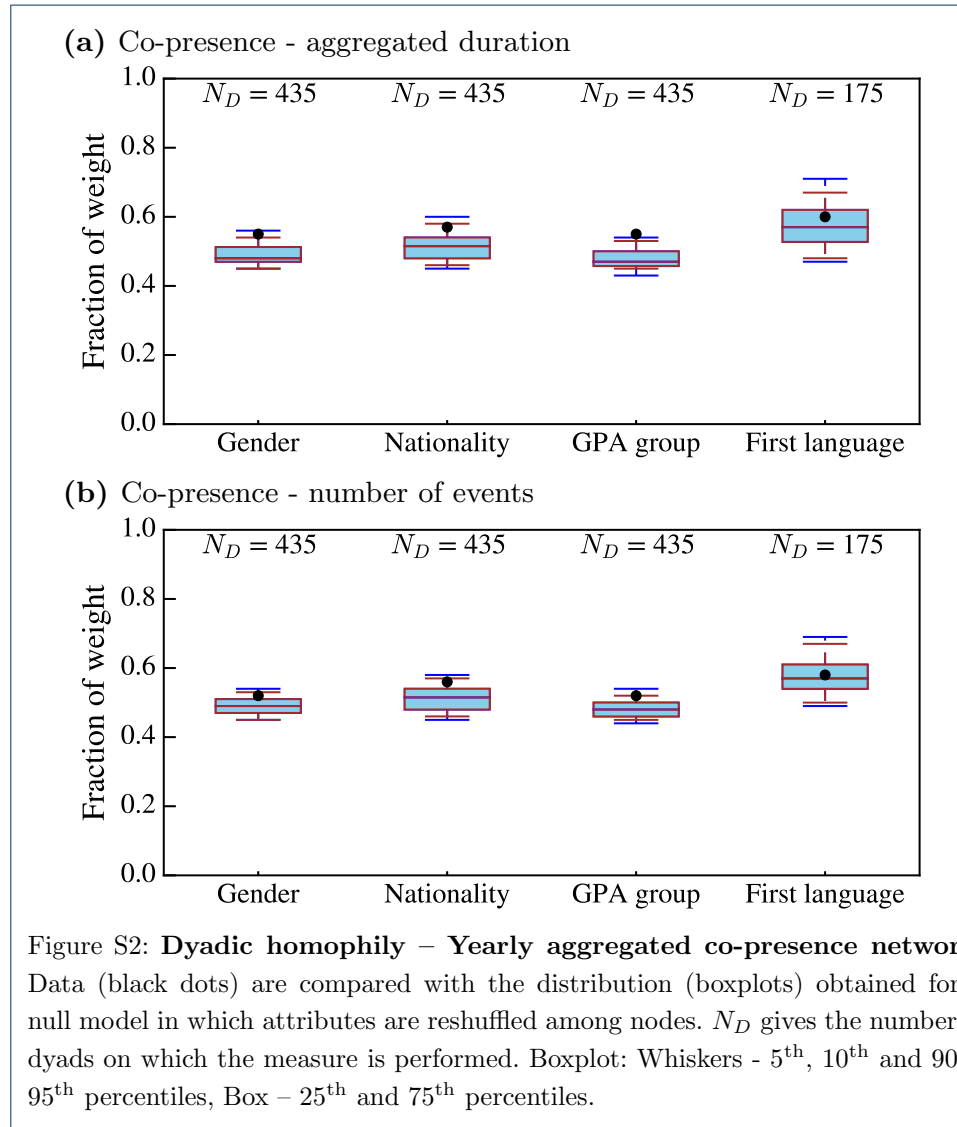

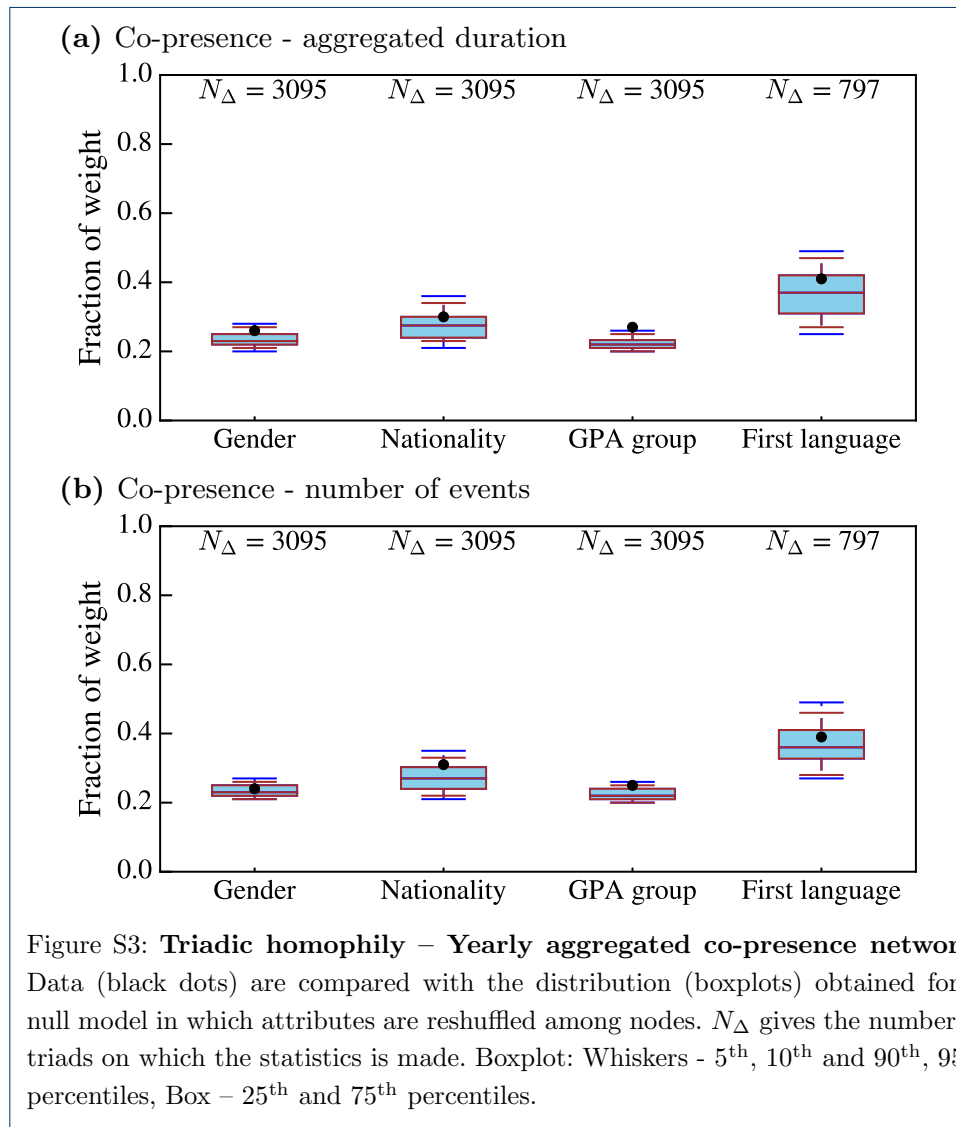

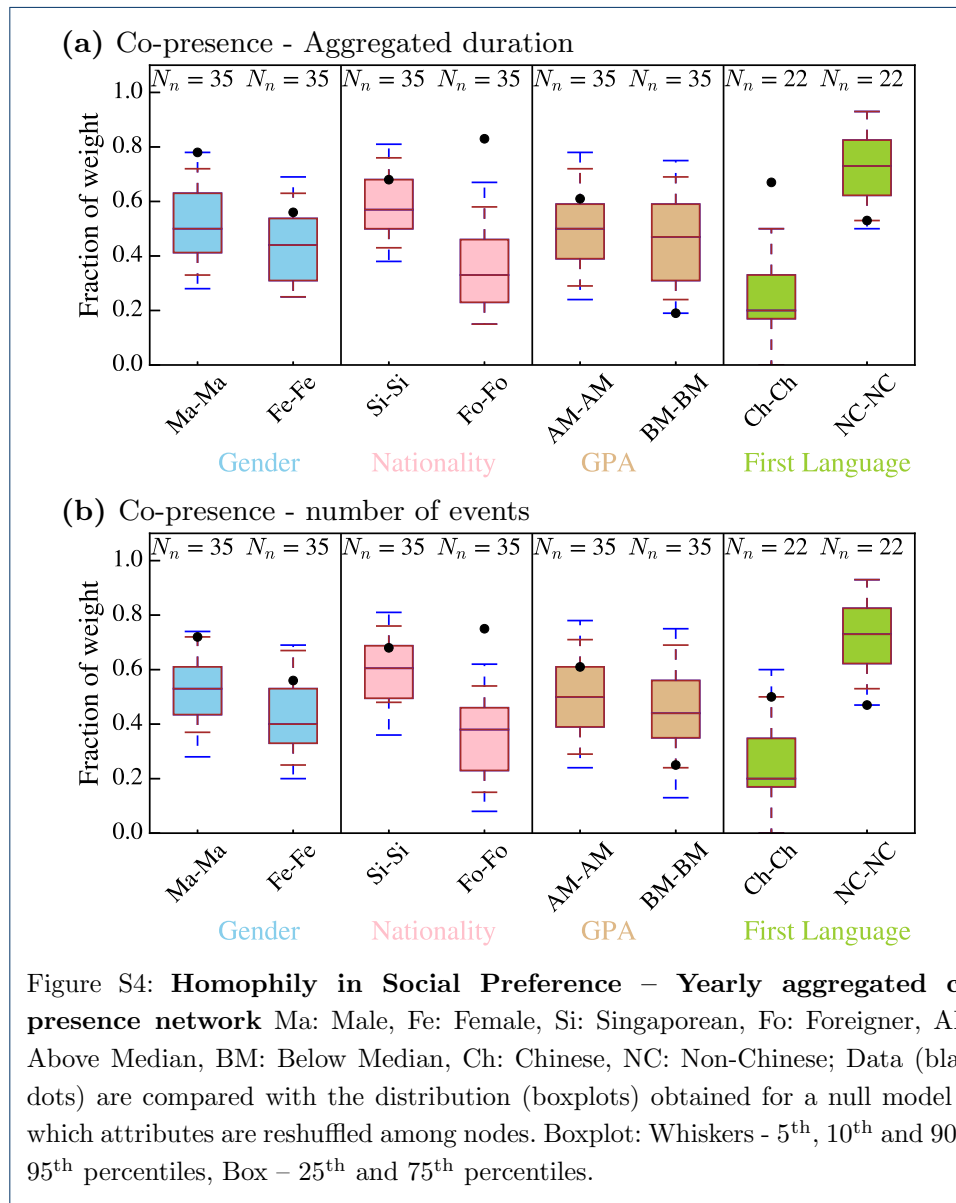

### 3 Evolution of homophily patterns in triads and social preference in the communication network

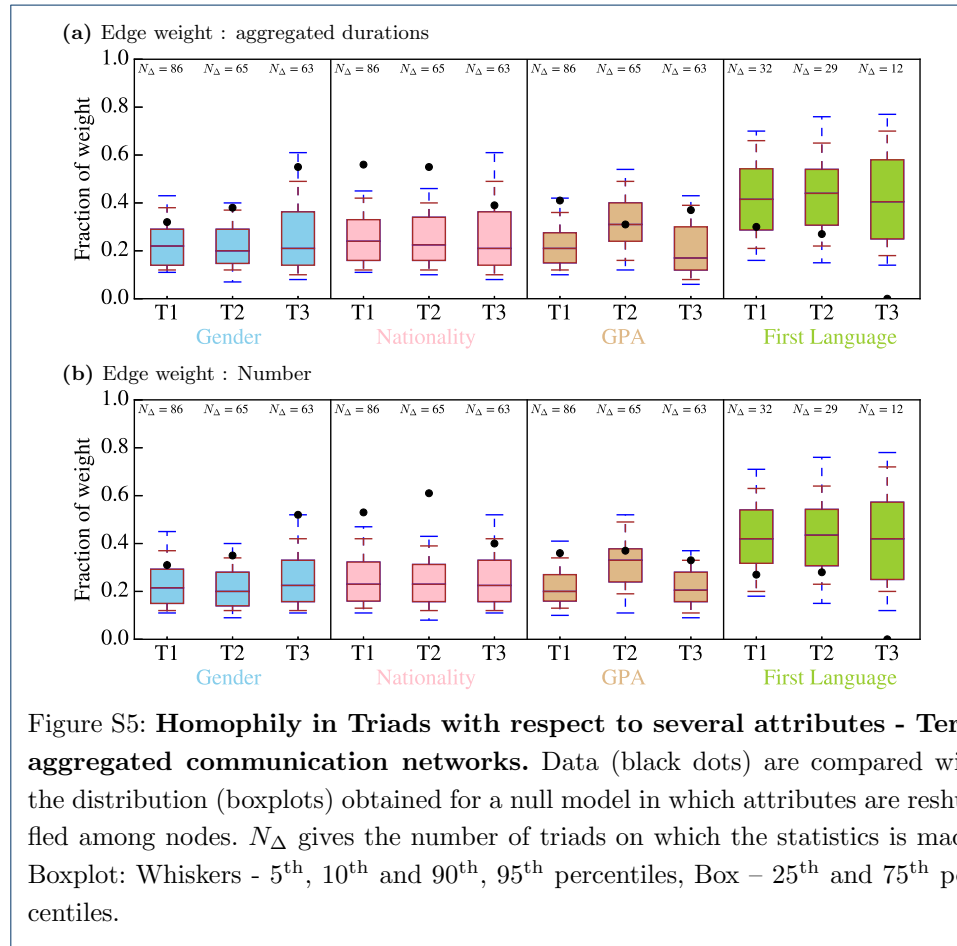

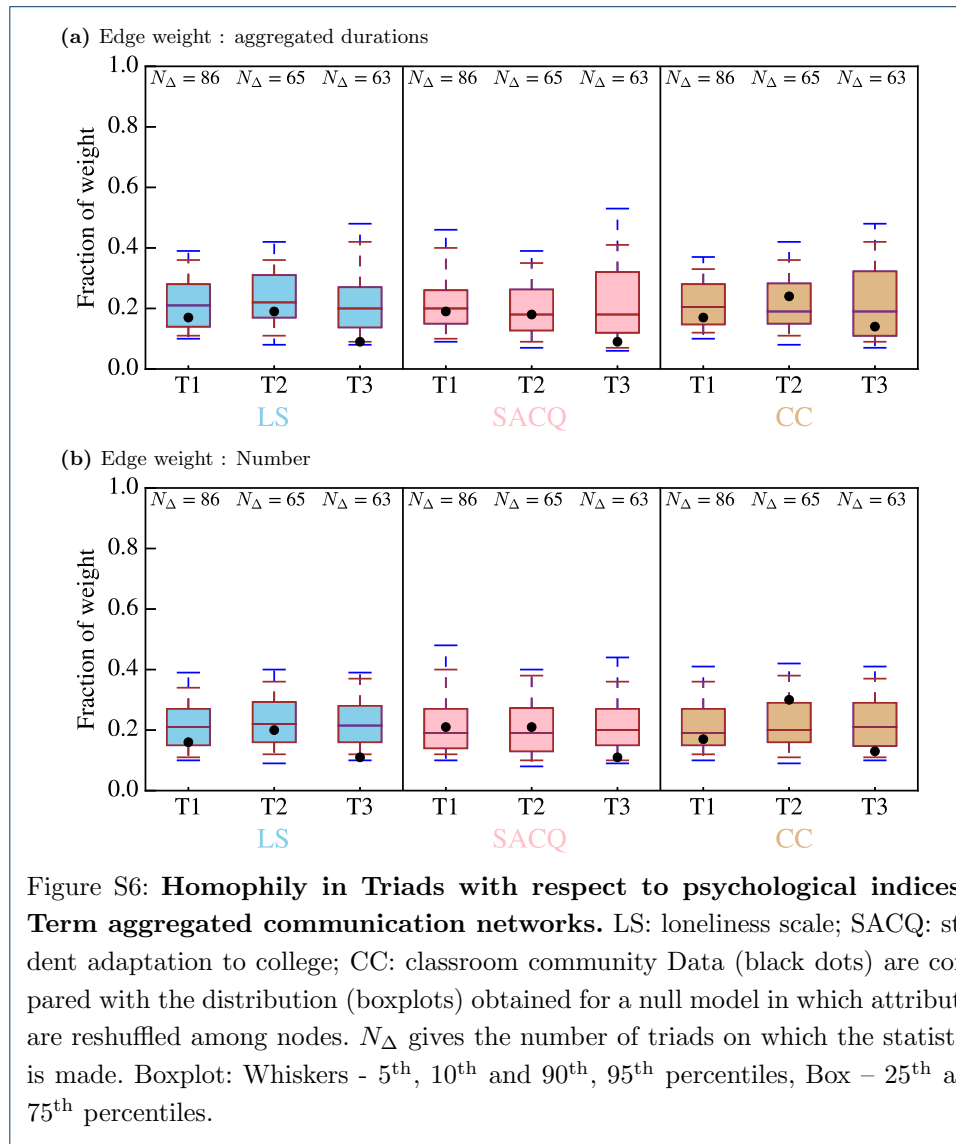

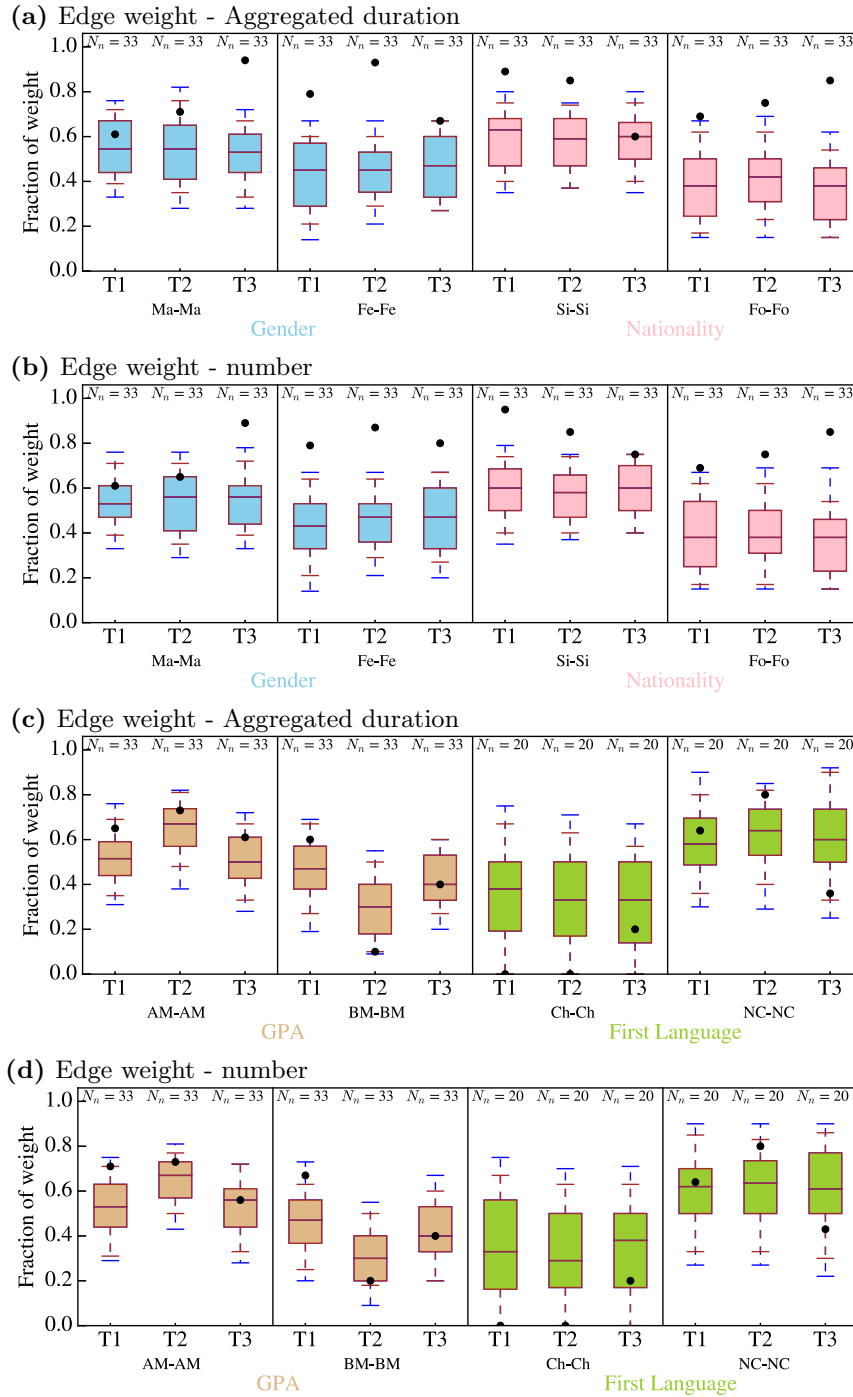

Figure S7: **Homophily in Social Preference with respect to several attributes - Term aggregated networks.** Ma: Male, Fe: Female, Si: Singaporean, Fo: Foreigner, AM: Above Median, BM: Below Median, Ch: Chinese, NC: Non-Chinese; Data (black dots) are compared with the distribution (boxplots) obtained for a null model in which attributes are reshuffled among nodes. Boxplot: Whiskers - 5<sup>th</sup>, 10<sup>th</sup> and 90<sup>th</sup>, 95<sup>th</sup> percentiles, Box - 25<sup>th</sup> and 75<sup>th</sup> percentiles.

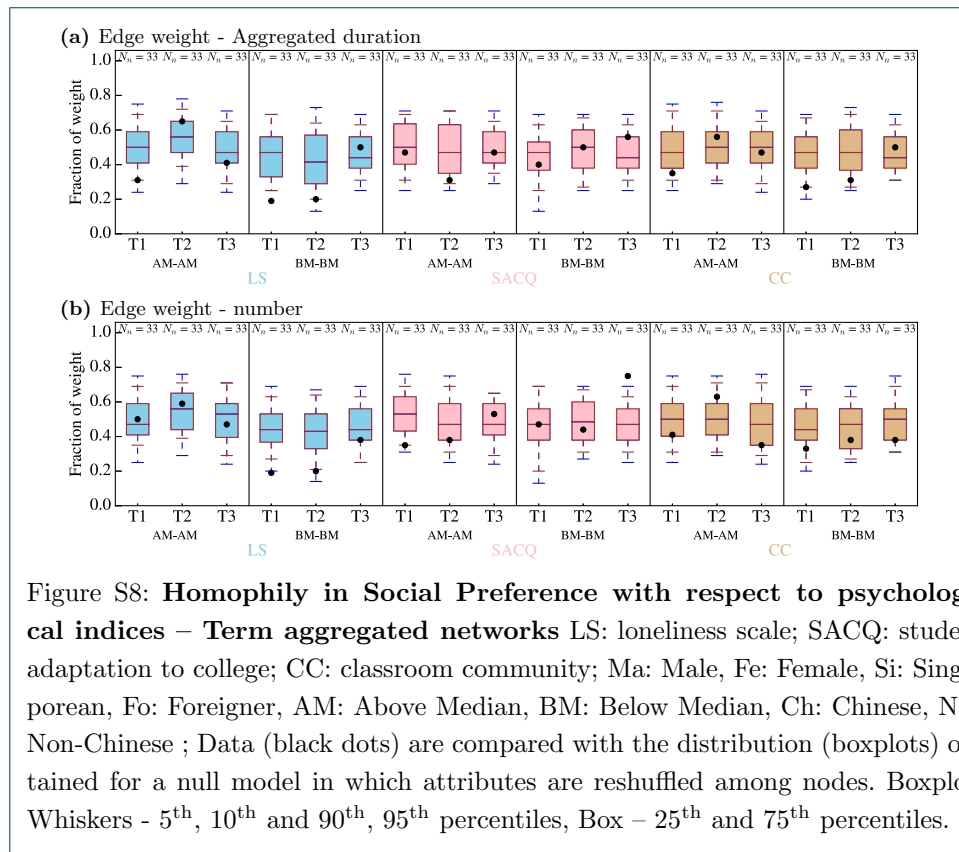

#### 4 Summary tables of homophily patterns for triads and social preferences

Table S2: Summary of the homophily patterns found in triads in the different networks, with respect to the various attributes considered.

| Attribute                     | Weight | Communication    |                  |                   | Co-presence       |                   |                   | Weight | Questionnaires |                  |                  |    |
|-------------------------------|--------|------------------|------------------|-------------------|-------------------|-------------------|-------------------|--------|----------------|------------------|------------------|----|
|                               |        | T1               | T2               | T3                | T1                | T2                | T3                |        | T0             | T1               | T2               | T3 |
| Gender                        | Volume | W                | S                | S                 | W                 | No                | VS                | Q1     | VS             | VS               | VS               | W  |
|                               | Number | W                | S                | S                 | No                | No                | VS                | Q2     | VS             | No               | VS               | VS |
| Nationality                   | Volume | VS               | VS               | W                 | VS                | No                | No                | Q1     | No             | No               | No               | No |
|                               | Number | VS               | VS               | W                 | VS                | No                | No                | Q2     | S              | No               | No               | No |
| GPA                           | Volume | S                | No               | W                 | S                 | VS                | S                 | Q1     | No             | S                | W                | No |
|                               | Number | S                | No               | W                 | No                | VS                | W                 | Q2     | No             | VS               | No               | W  |
| First Language                | Volume | No               | W <sub>het</sub> | VS <sub>het</sub> | No                | No                | No                | Q1     | No             | W <sub>het</sub> | W <sub>het</sub> | No |
|                               | Number | W <sub>het</sub> | W <sub>het</sub> | VS <sub>het</sub> | No                | No                | No                | Q2     | No             | No               | W <sub>het</sub> | No |
| Loneliness                    | Volume | No               | No               | S                 | VS <sub>het</sub> | No                | No                | Q1     | VS             | No               | No               | No |
|                               | Number | No               | No               | S                 | VS <sub>het</sub> | No                | No                | Q2     | No             | No               | No               | No |
| Student adaptation to college | Volume | No               | No               | W                 | W                 | VS <sub>het</sub> | VS <sub>het</sub> | Q1     | S              | No               | No               | No |
|                               | Number | No               | No               | W                 | W                 | No                | S <sub>het</sub>  | Q2     | W              | No               | No               | No |
| Classroom Community           | Volume | No               | No               | No                | No                | No                | No                | Q1     | No             | No               | No               | No |
|                               | Number | No               | W                | W <sub>het</sub>  | W                 | No                | No                | Q2     | No             | No               | No               | No |

Table S3: **Summary of the homophily patterns found in Social preferences in the different networks, with respect to the various attributes considered.** Ma: Male, Fe: Female, Si: Singaporean, Fo: Foreigner, AM: Above Median, BM: Below Median, Ch: Chinese, NC: Non-Chinese

| Attribute                     | Weight | Group | Communication     |                  |                  | Co-presence      |                   |                  | Weight | Questionnaires   |                   |                  |                   |
|-------------------------------|--------|-------|-------------------|------------------|------------------|------------------|-------------------|------------------|--------|------------------|-------------------|------------------|-------------------|
|                               |        |       | T1                | T2               | T3               | T1               | T2                | T3               |        | T0               | T1                | T2               | T3                |
| Gender                        | Volume | Ma    | No                | W                | VS               | No               | No                | W                | Q1     | No               | No                | No               | No                |
|                               |        | Fe    | VS                | VS               | W                | VS               | No                | No               |        | VS               | W                 | W                | S                 |
|                               | Number | Ma    | No                | No               | VS               | No               | No                | No               | Q2     | No               | No                | W                | VS                |
|                               |        | Fe    | VS                | VS               | VS               | S                | No                | No               |        | No               | VS                | No               | W                 |
| Nationality                   | Volume | Si    | VS                | VS               | No               | S                | No                | W <sub>het</sub> | Q1     | VS               | W                 | VS               | W                 |
|                               |        | Fo    | VS                | VS               | VS               | S                | No                | W                |        | VS               | S                 | W                | S                 |
|                               | Number | Si    | VS                | VS               | W                | S                | No                | W <sub>het</sub> | Q2     | VS               | S                 | VS               | W                 |
|                               |        | Fo    | VS                | VS               | VS               | W                | W                 | No               |        | VS               | VS                | S                | W                 |
| GPA                           | Volume | AM    | W                 | No               | No               | S                | W                 | S                | Q1     | W                | W                 | No               | No                |
|                               |        | BM    | W                 | W <sub>het</sub> | No               | No               | S <sub>het</sub>  | No               |        | W                | No                | No               | No                |
|                               | Number | AM    | W                 | No               | No               | W                | W                 | VS               | Q2     | No               | No                | W                | No                |
|                               |        | BM    | S                 | No               | No               | No               | VS <sub>het</sub> | W <sub>het</sub> |        | No               | No                | No               | VS                |
| First Language                | Volume | Ch    | W <sub>het</sub>  | W <sub>het</sub> | No               | W                | No                | W <sub>het</sub> | Q1     | S <sub>het</sub> | W <sub>het</sub>  | No               | S <sub>het</sub>  |
|                               |        | NC    | No                | W                | W <sub>het</sub> | No               | W <sub>het</sub>  | No               |        | W                | No                | No               | No                |
|                               | Number | Ch    | W <sub>het</sub>  | W <sub>het</sub> | No               | No               | W                 | W <sub>het</sub> | Q2     | W <sub>het</sub> | S <sub>het</sub>  | S <sub>het</sub> | W <sub>het</sub>  |
|                               |        | NC    | No                | W                | W <sub>het</sub> | No               | No                | No               |        | VS               | W                 | S                | VS                |
| Loneliness                    | Volume | AM    | W <sub>het</sub>  | No               | No               | No               | No                | No               | Q1     | No               | No                | No               | S <sub>het</sub>  |
|                               |        | BM    | VS                | W <sub>het</sub> | No               | W <sub>het</sub> | No                | S <sub>het</sub> |        | W                | VS <sub>het</sub> | No               | No                |
|                               | Number | AM    | No                | No               | No               | No               | No                | No               | Q2     | W <sub>het</sub> | No                | W <sub>het</sub> | VS <sub>het</sub> |
|                               |        | BM    | VS <sub>het</sub> | S <sub>het</sub> | No               | W <sub>het</sub> | No                | W <sub>het</sub> |        | VS               | W <sub>het</sub>  | No               | No                |
| Student adaptation to college | Volume | AM    | No                | W <sub>het</sub> | No               | VS               | No                | No               | Q1     | W <sub>het</sub> | No                | No               | S                 |
|                               |        | BM    | No                | No               | No               | W <sub>het</sub> | No                | No               |        | S                | No                | S                | No                |
|                               | Number | AM    | W                 | No               | No               | VS               | No                | No               | Q2     | S <sub>het</sub> | VS <sub>het</sub> | No               | No                |
|                               |        | BM    | No                | No               | VS               | W <sub>het</sub> | No                | W <sub>het</sub> |        | W <sub>het</sub> | VS <sub>het</sub> | No               | No                |
| Classroom Community           | Volume | AM    | W <sub>het</sub>  | No               | No               | VS               | VS                | No               | Q1     | W <sub>het</sub> | No                | No               | No                |
|                               |        | BM    | W <sub>het</sub>  | W <sub>het</sub> | No               | W <sub>het</sub> | VS <sub>het</sub> | W                |        | S <sub>het</sub> | W                 | No               | VS <sub>het</sub> |
|                               | Number | AM    | No                | W                | No               | VS               | S                 | No               | Q2     | W <sub>het</sub> | No                | No               | No                |
|                               |        | BM    | W <sub>het</sub>  | No               | No               | W <sub>het</sub> | W <sub>het</sub>  | W                |        | No               | VS                | No               | W <sub>het</sub>  |

## 5 Detailed tables of the numbers of concordant and discordant cases for each network pair

Table S4: Comparison of homophily in networks – A

(a) Communication vs. Co-presence

|               |            | Co-presence |   |   |    |           |           |            |
|---------------|------------|-------------|---|---|----|-----------|-----------|------------|
|               |            | VS          | S | W | No | $W_{het}$ | $S_{het}$ | $VS_{het}$ |
| Communication | VS         | 7           | 5 | 5 | 16 | 2         | 0         | 0          |
|               | S          | 2           | 2 | 1 | 6  | 0         | 0         | 0          |
|               | W          | 3           | 3 | 3 | 8  | 4         | 2         | 0          |
|               | No         | 8           | 2 | 8 | 32 | 9         | 2         | 3          |
|               | $W_{het}$  | 1           | 0 | 5 | 17 | 3         | 3         | 1          |
|               | $S_{het}$  | 0           | 0 | 0 | 2  | 0         | 0         | 0          |
|               | $VS_{het}$ | 0           | 0 | 0 | 2  | 1         | 0         | 0          |

(b) Communication vs. Q1

|               |            | Q1 |   |   |    |           |           |            |
|---------------|------------|----|---|---|----|-----------|-----------|------------|
|               |            | VS | S | W | No | $W_{het}$ | $S_{het}$ | $VS_{het}$ |
| Communication | VS         | 10 | 8 | 9 | 7  | 0         | 0         | 1          |
|               | S          | 2  | 3 | 3 | 3  | 0         | 0         | 0          |
|               | W          | 3  | 1 | 4 | 15 | 0         | 0         | 0          |
|               | No         | 1  | 4 | 6 | 45 | 2         | 4         | 2          |
|               | $W_{het}$  | 0  | 0 | 2 | 22 | 6         | 0         | 0          |
|               | $S_{het}$  | 0  | 0 | 0 | 2  | 0         | 0         | 0          |
|               | $VS_{het}$ | 0  | 0 | 0 | 2  | 0         | 0         | 1          |

(c) Communication vs. Q2

|               |            | Q2 |   |   |    |           |           |            |
|---------------|------------|----|---|---|----|-----------|-----------|------------|
|               |            | VS | S | W | No | $W_{het}$ | $S_{het}$ | $VS_{het}$ |
| Communication | VS         | 13 | 6 | 8 | 7  | 1         | 0         | 0          |
|               | S          | 7  | 0 | 1 | 3  | 0         | 0         | 0          |
|               | W          | 1  | 2 | 5 | 14 | 0         | 0         | 1          |
|               | No         | 3  | 0 | 6 | 44 | 6         | 0         | 5          |
|               | $W_{het}$  | 4  | 0 | 2 | 16 | 4         | 4         | 0          |
|               | $S_{het}$  | 0  | 0 | 0 | 2  | 0         | 0         | 0          |
|               | $VS_{het}$ | 0  | 0 | 0 | 2  | 1         | 0         | 0          |

Table S5: **Comparison of homophily in networks - B**(a) **Co-presence vs. Q1**

|           |                   | Co-presence |    |   |    |                  |                  |                   |
|-----------|-------------------|-------------|----|---|----|------------------|------------------|-------------------|
|           |                   | VS          | S  | W | No | W <sub>het</sub> | S <sub>het</sub> | VS <sub>het</sub> |
| Coproence | VS                | 5           | 0  | 8 | 8  | 0                | 0                | 0                 |
|           | S                 | 1           | 3  | 4 | 3  | 1                | 0                | 0                 |
|           | W                 | 1           | 3  | 3 | 11 | 2                | 0                | 2                 |
|           | No                | 9           | 10 | 5 | 52 | 5                | 2                | 0                 |
|           | W <sub>het</sub>  | 0           | 0  | 4 | 11 | 0                | 2                | 2                 |
|           | S <sub>het</sub>  | 0           | 0  | 0 | 7  | 0                | 0                | 0                 |
|           | VS <sub>het</sub> | 0           | 0  | 0 | 4  | 0                | 0                | 0                 |

(b) **Coproence vs. Q2**

|           |                   | Q1 |   |   |    |                  |                  |                   |
|-----------|-------------------|----|---|---|----|------------------|------------------|-------------------|
|           |                   | VS | S | W | No | W <sub>het</sub> | S <sub>het</sub> | VS <sub>het</sub> |
| Coproence | VS                | 6  | 0 | 3 | 10 | 0                | 0                | 2                 |
|           | S                 | 5  | 2 | 1 | 4  | 0                | 0                | 0                 |
|           | W                 | 3  | 1 | 7 | 7  | 2                | 2                | 0                 |
|           | No                | 11 | 4 | 9 | 49 | 6                | 2                | 2                 |
|           | W <sub>het</sub>  | 3  | 1 | 2 | 7  | 4                | 0                | 2                 |
|           | S <sub>het</sub>  | 0  | 0 | 0 | 7  | 0                | 0                | 0                 |
|           | VS <sub>het</sub> | 0  | 0 | 0 | 4  | 0                | 0                | 0                 |

(c) **Q1 vs. Q2**

|    |                   | Q2 |   |    |    |                  |                  |                   |
|----|-------------------|----|---|----|----|------------------|------------------|-------------------|
|    |                   | VS | S | W  | No | W <sub>het</sub> | S <sub>het</sub> | VS <sub>het</sub> |
| Q1 | VS                | 8  | 2 | 4  | 2  | 0                | 0                | 0                 |
|    | S                 | 8  | 0 | 4  | 4  | 0                | 0                | 0                 |
|    | W                 | 6  | 4 | 4  | 10 | 0                | 0                | 0                 |
|    | No                | 6  | 2 | 10 | 68 | 4                | 2                | 4                 |
|    | W <sub>het</sub>  | 0  | 0 | 0  | 4  | 2                | 2                | 0                 |
|    | S <sub>het</sub>  | 0  | 0 | 0  | 0  | 2                | 0                | 2                 |
|    | VS <sub>het</sub> | 0  | 0 | 0  | 0  | 4                | 0                | 0                 |
